# Supplementary material for: EnCortex: A General, Extensible and Scalable Framework for Decision Management in New-age Energy Systems
Source: arXiv:2503.06959 source file (2025-03-10)
Supplement: Supplementary file 1 [file supp_uncert.tex]

In this part of the section, we explore how our optimizers perform with varying forecasting methods. Specifically, we explore optimizing for cost and carbon savings with MILP and DQN as our optimizers on six forecasting methods, stated in \ref{sec:infra_components}. From Table \ref{tab:milp_dqn_for_forecasts_ba}, we observe two ends of the forecasting error spectrum, where the range of MAE is relatively lower for all forecasting methods for price forecasting as opposed to carbon forecasting, arising from the fact that the time-series of carbon emissions lack seasonality and is often harder to predict, as depicted by the performance of LightGBM and N-BEATS on the dataset. While the DQN-RL optimizer comfortably outperforms MILP in cost savings, it slightly lags behind MILP in carbon savings, likely caused due to the fact that accounting for high uncertainty is a much more difficult task for the DQN-RL optimizer.

% Optimization - MILP vs RL
\begin{table}[h]
\centering
\scalebox{0.8}{
\begin{tabular}{|c|c|c| c|}
\hline
      \textbf{Objective}& \textbf{Algorithm} & \multicolumn{2}{|c|}{\textbf{Savings}} \\\cline{3-4}
     & & Cost & Carbon \\ 
     & &  (in EUR) &  (in gCO2eq)\\ \hline
     Cost  & DQN & \textbf{117727.62} & -59906.70 \\
     Optimization & MILP & 116106.74 & -42720.57  \\ \hline
     Carbon  & DQN& -15347.10 &211594.86\\
     Optimization & MILP& -8687.30 & \textbf{227272.49} \\ \hline
     Joint  & DQN & 81545.06 & 137774.50\\
     Optimization($\alpha=1.115$) &MILP & 74898.32 & \textbf{164751.74} \\ \hline
\end{tabular}
}
\caption{Savings across different Objectives when forecasts are very accurate. Takeaway: Depending on the input forecast data, RL performs better in price-optimization while MILP better in the other two objectives on the mean forecast data.}
\label{tab:diff_obj_actual}
\end{table}

\begin{table}[h]
\centering
\scalebox{0.8}{
\begin{tabular}{|c|c|c| c|}
    \hline
      \textbf{Objective}& \textbf{Algorithm} & \multicolumn{2}{|c|}{\textbf{Savings}} \\\cline{3-4}
     & & Cost & Carbon \\ 
     & &  (in EUR) &  (in gCO2eq)\\ \hline
     Cost  & DQN & 85177.23 & -82077.83  \\
     Optimization & MILP & \textbf{88198.84} & -43539.75  \\ \hline
     Carbon  & DQN& -36437.6 & 140219.63\\
     Optimization & MILP& -6016.38 & \textbf{163336.50}  \\ \hline
     Joint  & DQN & 24902.34& 92623.95 \\
     Optimization($\alpha=1.155$) &MILP &  46272.44& 135897.29  \\ \hline
\end{tabular}
}
\caption{Savings across different Objectives when mean of previous 10 days' actual values are used as forecasts. Imp: We chose $\alpha$ from the pareto optimal points in the further plot to compare apples to apples}
\label{tab:diff_obj_mean}
\end{table}

\begin{table*}[hbtp]
\caption{Cost and carbon savings of two optimizers on different forecasting methods, each with varying mean average error(MAE).}
\scalebox{0.8}{
\begin{tabular}{|c|cc|cc|cc|}
\hline
Forecast Method & \multicolumn{2}{c|}{Forecasting MAE} & \multicolumn{2}{c|}{Cost Savings(K)}                 & \multicolumn{2}{c|}{Carbon Emission Savings($kgCO_2eq$)}     \\ \cline{2-7} 
                & \multicolumn{1}{c|}{Price}  & Carbon & \multicolumn{1}{c|}{MILP}          & DQN             & \multicolumn{1}{c|}{MILP}             & DQN             \\ \hline
Accurate        & \multicolumn{1}{c|}{0}      & 0      & \multicolumn{1}{c|}{116.1}         & \textbf{117.73} & \multicolumn{1}{c|}{\textbf{227.27}}  & 211.59          \\ \hline
Noise           & \multicolumn{1}{c|}{19.82}  & 19.08  & \multicolumn{1}{c|}{44.64}         & \textbf{57.86}  & \multicolumn{1}{c|}{123.93}           & \textbf{163.17} \\ \hline
Yesterday       & \multicolumn{1}{c|}{9.70}   & 42.19  & \multicolumn{1}{c|}{77.74}         & \textbf{83.08}  & \multicolumn{1}{c|}{\textbf{138.384}} & 129.37          \\ \hline
Mean            & \multicolumn{1}{c|}{9.94}   & 48.13  & \multicolumn{1}{c|}{\textbf{88.2}} & 83.24           & \multicolumn{1}{c|}{\textbf{163.34}}  & 135.06          \\ \hline
LightGBM        & \multicolumn{1}{c|}{11.88}  & 38.33  & \multicolumn{1}{c|}{55.89}         & \textbf{62.14}  & \multicolumn{1}{c|}{124.4}            & \textbf{128.73} \\ \hline
N-BEATS         & \multicolumn{1}{c|}{10.13}  & 38.49  & \multicolumn{1}{c|}{73.3}          & \textbf{76.71}  & \multicolumn{1}{c|}{\textbf{145.82}}  & 130.94          \\ \hline
\end{tabular}
}
\label{tab:milp_dqn_for_forecasts_ba}
\end{table*}
